# Supplementary material for: Leveraging Synthetic Adult Datasets for Unsupervised Infant Pose Estimation
Source: arXiv:2504.05789 source file (2025-04-08)
Supplement: Supplementary file 1 [file X_suppl.tex]

\documentclass[10pt,twocolumn,letterpaper]{article}

\usepackage{cvpr}              % To produce the CAMERA-READY version

\input{preamble}

%%%%%%%%% PAPER ID  - PLEASE UPDATE
 % *** Enter the Paper ID here

\title{Supplementary Material for \ours{}}

\begin{document}
\maketitle
\input{sec/supp/supp}
%\clearpage
%\newpage
{
    \small
    \bibliographystyle{ieeenat_fullname}
    \bibliography{bib/shift}
}

\end{document}
